# Supplementary material for: Estimating Noisy Class Posterior with Part-level Labels for Noisy Label Learning
Source: arXiv:2405.05714 source file (2024-07-02)
Supplement: Supplementary file 1 [file X_suppl.tex]

\clearpage
\appendix
\setcounter{page}{1}
\maketitlesupplementary
\section{Classifier training with PLM}
In Eq. (4) of main paper, we discussed the empirical risk for estimating the noisy class posterior and the single-to-multiple transition matrix. In this supplementary material, we will provide a detailed discussion on how to train a robust classifier using PLM and loss correction \cite{patrini2017making} techniques.

As discussed in the main paper, the classification task aims to learn a classifier $f:\mathcal{X} \rightarrow \mathcal{C}$ that maps each instance $\boldsymbol{x}_i$ to its corresponding label $y_i$. Given the network for estimating the clean class posterior as $g: \mathcal{X} \rightarrow \mathcal{R}^c$, the classifier can be represented as follows: $f(\boldsymbol{x})=\arg\max_{i \in \{1,\cdots,c\}}{g_i(\boldsymbol{x})}$. Here, $g_i(\boldsymbol{x})$ refers to the $i$-th element of the vector $g(\boldsymbol{x})$, which represents the estimated probability $\hat{P}(Y=i|X=\boldsymbol{x})$. Given a noisy dataset $\tilde{\mathcal{D}} = \{(\boldsymbol{x}_i,\tilde{y_i})\}_{i=1}^n$, the empirical risk of the classifier is defined as:
\begin{equation}
  \tilde{R}(f)=\frac{1}{n}\sum_{i=1}^{n}\ell_1(f(\boldsymbol{x}_i),\tilde{y}_i),
\end{equation}
where $\ell_1$ denotes a classification loss. 
Loss correction methods typically introduce a transition matrix $T(\boldsymbol{x})$ to establish a connection between the posterior of the noisy and clean classes. This allows training a clean classifier by minimizing the empirical risk with noisy dataset. Based on previous loss correction methods, the noise transition matrix $T(\boldsymbol{x})$ can be estimated, and we have $P(\boldsymbol{\tilde{Y}}|X=\boldsymbol{x}) = T(\boldsymbol{x})P(\boldsymbol{Y}|X=\boldsymbol{x})$. Let the noisy class posterior estimation network be denoted as $g^e: \mathcal{X} \rightarrow \mathcal{R}^c$ where $g^e_i(\boldsymbol{x})=P(\tilde{Y}=i|X=\boldsymbol{x})$. The noisy class classifier $f^e(\boldsymbol{x})$ can be represented as:
\begin{equation}
  f^e(\boldsymbol{x})=\arg\max_{i \in \{1,\cdots,c\}}{g^e_i(\boldsymbol{x})}=\arg\max_{i \in \{1,\cdots,c\}}(T(\boldsymbol{x})g)_i(\boldsymbol{x}).
  \label{eq:eqfe}
\end{equation}
Therefore, the empirical risk in loss correction methods can be expressed as:
\begin{equation}
  \tilde{R}(g)=\frac{1}{n}\sum_{i=1}^{n}\ell_1(f^e(\boldsymbol{x}_i),\tilde{y}_i).
\end{equation}
By minimizing this loss it is possible to construct algorithms with classifier-consistency.

% Similarly, given a dataset $\{(\boldsymbol{x}_i,\boldsymbol{y}_i)\}_{i=1}^n$ with multiple part-level labels, the empirical risk can be represented as follows:
% \begin{equation}
%   R^\prime(f)=\frac{1}{n}\sum_{i=1}^{n}\ell_2(f(\boldsymbol{x}_i),\boldsymbol{y}^\prime_i),
% \end{equation}
% where $\ell_2$ denotes a multi-label classification loss. 

We denote the mapping $g^p: \mathcal{X} \rightarrow \mathcal{R}^c$ where $g^p_i(\boldsymbol{x})=P(Y^\prime_i=1|X=\boldsymbol{x})$. Given the single-to-multiple transition matrix $U(\boldsymbol{x})$ where $U_{ij}(\boldsymbol{x})=P(Y^\prime_j=1|\tilde{Y}=i, X=\boldsymbol{x})$, the part-level multi-label classifier $f^p(\boldsymbol{x})$ can be represented as:
\begin{equation}
  \begin{aligned}
    f^p(\boldsymbol{x}) &= \{i|g^p_i(\boldsymbol{x}) > \frac{1}{2}\}=\{i|(U(\boldsymbol{x})g^e)_i(\boldsymbol{x}) > \frac{1}{2}\} \\
    &= \{i|(U(\boldsymbol{x})T(\boldsymbol{x})g)_i(\boldsymbol{x}) > \frac{1}{2}\}.
  \end{aligned}
\end{equation}
Similarly, given a dataset $\{(\boldsymbol{x}_i,\boldsymbol{y}_i)\}_{i=1}^n$ with multiple part-level labels, the empirical risk of the training with part-level labels is defined as:
\begin{equation}
  R^\prime(f^p)=\frac{1}{n}\sum_{i=1}^{n}\ell_2(f^p(\boldsymbol{x}_i),\boldsymbol{y}^\prime_i).
\end{equation}
where $\ell_2$ denotes a multi-label classification loss. 

Then, the empirical risk of the joint training framework is defined as:
\begin{equation}
    \begin{aligned}
        \hat{R}(g,f^p)&=\frac{1}{2}(\tilde{R}(g)+R^\prime(f^p))\\
        &= \frac{1}{2n}\sum_{i=1}^{n}[\ell_1(f^e(\boldsymbol{x}_i),\tilde{y}_i)+\ell_2(f^p(\boldsymbol{x}_i),\boldsymbol{y}^\prime_i)]. \label{eq:risk}
    \end{aligned}
\end{equation}
We minimize the empirical risk to obtain a robust classifier. The training process for the single-to-multiple transition matrix is depicted in Figure \ref{fig:meth1}, in which we achieve it by minimizing the empirical risk defined in Eq. (4) of the main paper. The training of the classifier is illustrated in Figure \ref{fig:meth2}, where we keep the trained matrix estimation network fixed and combine it with the noise transition matrix obtained through existing loss correction methods. We then optimize the empirical risk discussed before for training. The training procedure is outlined concisely in Algorithm \ref{alg:algorithm}.

\begin{algorithm}[tb]
    \caption{PLM training framework}
    \label{alg:algorithm}
    \begin{algorithmic}[1]
        \REQUIRE Noisy training dataset $\mathcal{D}$, noise transition matrix $T(\boldsymbol{x})$ derived from existing methods.\\
        \ENSURE Classifier model $f$.
        \STATE Minimize a classification loss to learn a labeling classifier $f^l$ from $\mathcal{D}$.
        \STATE Obtain the set of sub-instances $\mathcal{S}$ by cropping the instances in $\mathcal{D}$.
        \STATE Construct multi-labels by using $f^l$ to label the sub-instances in $\mathcal{S}$.
        \STATE Train a single-to-multiple transition matrix estimation network $g^u$ by minimizing the loss defined in Equation (4) of the main paper.
        \STATE Fix the parameters of $g^u$, set $g^e(\boldsymbol{x}) = (T(\boldsymbol{x})g)(\boldsymbol{x})$, then minimize the Equation (4) with updated $g^u$ to optimize $g$.
        \STATE Obtain the classifier $f(\boldsymbol{x})=\arg\max_{i \in \{1,\cdots,c\}}{g_i(\boldsymbol{x})}$. Here, $g_i(\boldsymbol{x})$ represents the $i$-th element of the network output vector $g(\boldsymbol{x})$.
        \STATE \textbf{return} Optimized classifier $f$.
    \end{algorithmic}
\end{algorithm}

\begin{figure*}[t]
  \centering
  \begin{minipage}[t]{\linewidth}
    \centering
    \begin{minipage}[t]{0.42\linewidth}
      \centering
      \includegraphics[height=5cm]{./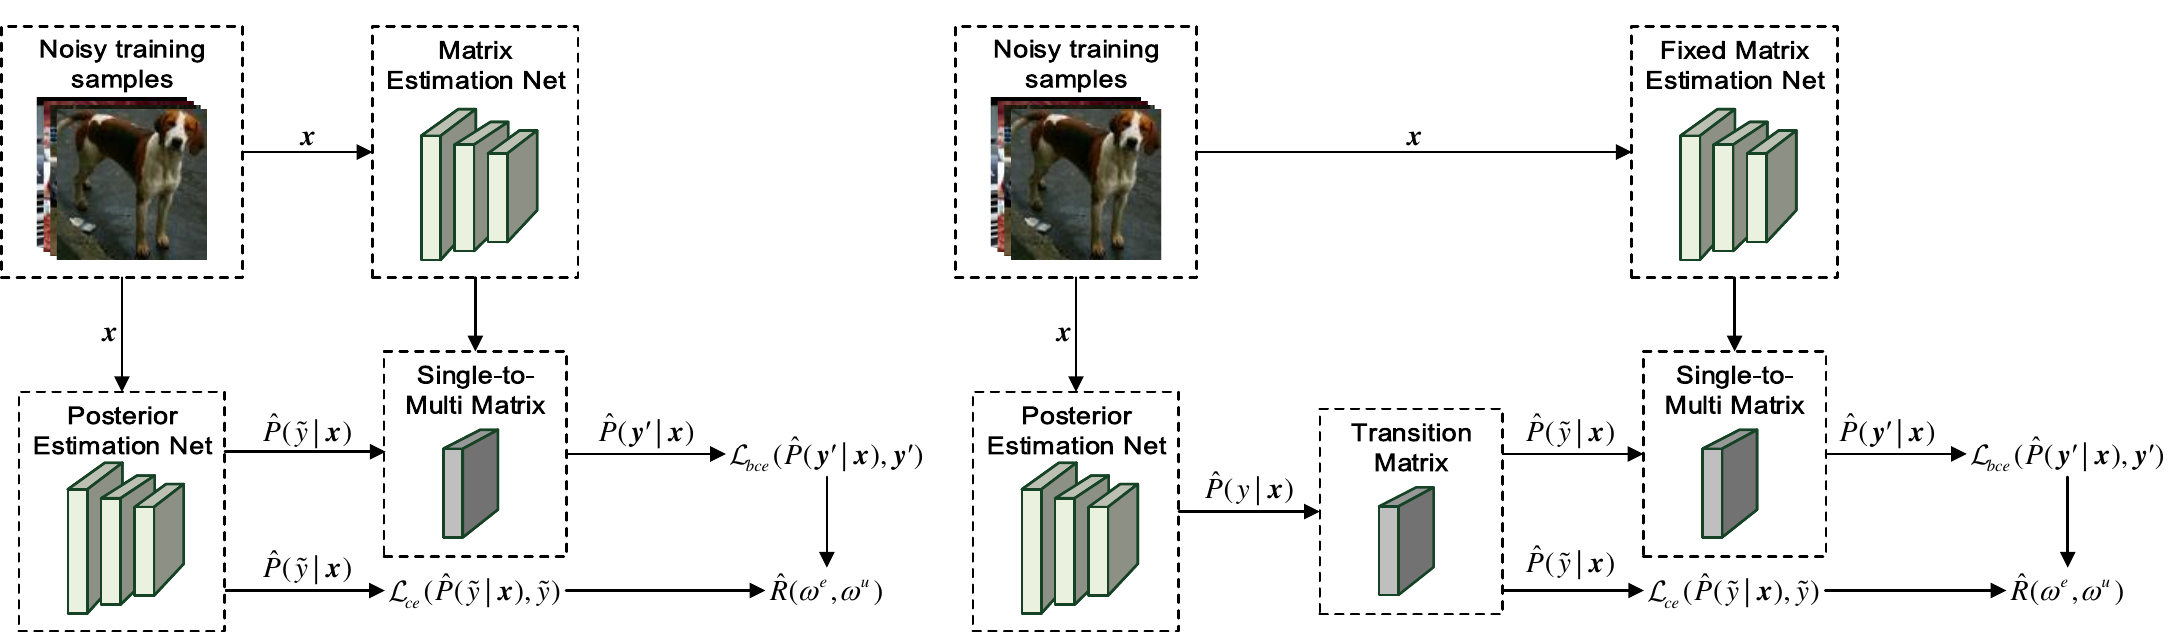}
      \subcaption{}\label{fig:meth1}
    \end{minipage}
    \begin{minipage}[t]{0.57\linewidth}
      \centering
      \includegraphics[height=5cm]{./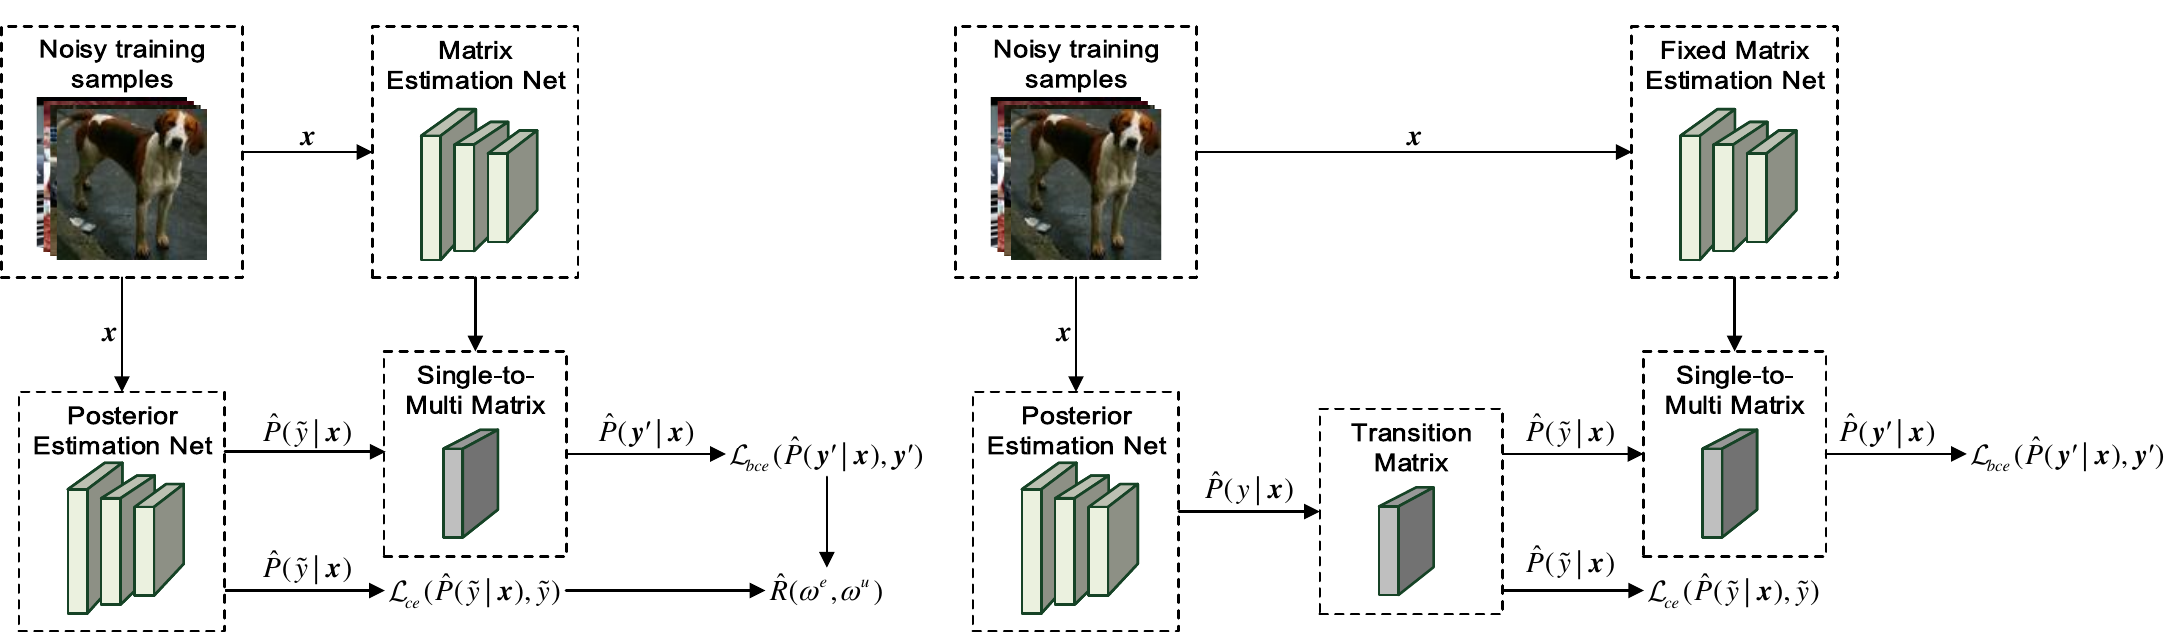}
      \subcaption{}\label{fig:meth2}
    \end{minipage}
  \end{minipage}
  \caption{Illustration of neural network training using PLM. The parameters for the posterior estimation network and the single-to-multiple matrix estimation network are denoted as $\omega^e$ and $\omega^u$, respectively. (a) Utilizing PLM for estimating the noisy class posterior while simultaneously training the matrix estimation network. (b) Fixing the matrix estimation network and integrating loss correction method to facilitate LNL.}
\end{figure*} 

% \begin{algorithm}[t]
% 	\caption{Classifier training with PLM.}
% 	\label{alg:algorithm1}
% 	\KwIn{Noisy Datasets $\tilde{\mathcal{D}} = \{(\boldsymbol{x}_i,\tilde{y_i})\}_{i=1}^n$.}
% 	\KwOut{Labels of nodes in query set of $\mathcal{T}_{mt}$.}  
% 	\BlankLine
% 	% Initialize $\bm{\theta}$ randomly;
	
% 	\While{\textnormal{not converged}}{
% 		Sample batch of meta-training tasks $\mathcal{T}_{i} \sim p(\mathcal{T})$;
		
% 		\ForEach{task in $\mathcal{T}_{i}$}{
%       P
% 			% Evaluate $\mathcal{L}_{\mathcal{T}_{i}}\left(f_{\bm{\theta}}\right)$ using $\mathcal{S}_{i}$;
			
% 			% Compute adapted parameters $\bm{{\theta}^{\prime}_{i}}$;
			
% 			% Evaluate $\mathcal{L}_{\mathcal{T}_{i}}\left(f_{\bm{{\theta}_{i}^{\prime}}}\right)$ using $\mathcal{Q}_{i}$;
% 		}
% 		% Update $\bm{\theta}$ by; 
% 	}
	
% 	% Compute adapted parameters $\bm{{\theta}^{\prime}_{mt}}$ using support set of $\mathcal{T}_{mt}$; 
	
% 	% Predict labels of nodes in query set of $\mathcal{T}_{mt}$ using model $f_{\bm{{\theta}_{mt}^{\prime}}}$.

% \end{algorithm}
\section{Identifiability of single-to-multiple transition matrix}
In this paper, we introduce a brand-new single-to-multiple transition matrix. In this section, we will discuss the identifiability of this transition matrix. Specifically, regarding $P(\boldsymbol{Y}^\prime|\boldsymbol{x}) = U(\boldsymbol{x})P(\tilde {\boldsymbol{Y}}|\boldsymbol{x})$, when the matrix $U(\boldsymbol{x})$ is unconstrained, the following issue arises: there exists an infinite number of non-singular matrices $Q \in \mathbb{R}^{c \times c}$ such that 
\begin{equation}
    P(\boldsymbol{Y}^\prime|\boldsymbol{x}) = (U(\boldsymbol{x})Q)(Q^{-1}P(\tilde {\boldsymbol{Y}}|\boldsymbol{x})). 
\end{equation}
This situation emerges from the network training process in joint training framework of Section 3.4: 
\begin{equation}
    g^p(\boldsymbol{x})=g^u(\boldsymbol{x})g^e(\boldsymbol{x}), 
\end{equation}
where $g^p(\boldsymbol{x})$, $g^e(\boldsymbol{x})$ and $g^u(\boldsymbol{x})$ correspond to the estimates of part-level labels, noisy class posterior, and the matrix respectively. The specific concern appears to center on the scenario where $g^p(\boldsymbol{x})=\hat P(\boldsymbol{Y}^\prime|\boldsymbol{x})$ and $g^e(\boldsymbol{x}) = Q^{-1} \hat{P}(\tilde {\boldsymbol{Y}}|\boldsymbol{x})$, yielding $g^u(\boldsymbol{x}) = U (\boldsymbol{x})Q \neq U(\boldsymbol{x})$.

In this paper, we employ joint training to simultaneously utilize noisy labels and part-level labels for optimizing both $g^e$ and $g^p$. More precisely, $g^e$ is directly guided by $\tilde Y$, aligning with a coarse $g^e(\boldsymbol{x}) = \hat{P}(\tilde{\boldsymbol{Y}}|\boldsymbol{x})$, while $g^p(\boldsymbol{x})$ is supervised by $Y^\prime$ to meet $g^p(\boldsymbol{x}) = \hat{P} (\boldsymbol{Y}^{\prime}| \boldsymbol{x})$. This dual supervision constrains $g^u(\boldsymbol{x})$ to comply with $\hat{P} (\boldsymbol{Y}^{\prime}| \boldsymbol{x}) = g^u(\boldsymbol{x}) \hat{P}(\tilde{\boldsymbol{Y}}|\boldsymbol{x})$, resulting in $g^u(\boldsymbol{x}) = \hat{U}(\boldsymbol{x})$. This means that the potential scenario, where $Q$ leads to $g^e(\boldsymbol{x}) = Q^{-1} \hat{P}(\tilde {\boldsymbol{Y}}|\boldsymbol{x})$ and then $g^u(\boldsymbol{x}) = \hat{U}(\boldsymbol{x})Q$, is preemptively negated through supervision from $\tilde Y$. Therefore, during training with the joint framework, the matrix's identifiability is ensured. This approach also echoes the matrix estimation strategy presented in MEIDTM \cite{cheng2022instance}.

\section{Analysis of time complexity}
In the main text, we introduced additional modules to aid in estimating the noisy class posterior, which to some extent increases the algorithm's time complexity. Therefore, in this section, we will discuss the time complexity and efficiency of the proposed method in comparison to our baseline model (Forward \cite{patrini2017making}).

Let us assume that the time complexity for training the baseline model for one epoch is denoted as $O(T)$, and the time complexity for making predictions on the entire training set is $O(P)$. Additionally, the introduction of an extra noise transition matrix layer contributes an additional time complexity of $O(E)$. Considering Forward as the baseline, the time complexity of the proposed method can be expressed as $O(e_1T+cP+e_2(2T+E)+e_3(T+P+2E))$, where $e_1$, $e_2$, and $e_3$ represent the number of epochs for the annotator, transition matrix estimator, and classifier training, respectively, and $c$ indicates the cropping frequency. Regarding the concerns raised about the additional transition matrix and cropping strategy, we would like to further elaborate: Firstly, the added complexity due to the training of the extra transition matrix estimation network is $O(e_2(2T+E))$. Secondly, since cropping strategies augment the sample count during annotation and not during training, the complexity increase is $O(5P)$, i.e., involving 5 rounds of annotation for all instances.

For comparison, the time complexity of the Forward method is expressed as $O(e_4T+P+e_5(T+E))$, where $e_4$ and $e_5$ represent the number of epochs for the anchor estimation network and classifier training, respectively. For the sake of facilitating comparison, we assume that each section underwent an equal number of training epochs $e$, i.e., $e=e1=e2=e3=e4=e5$. The complexity of the proposed method is represented as $O(4eT + (c+e)P + (1+2e)E)$, whereas the complexity of the Forward method is denoted as $O(2eT + P + eE)$. Consider the transition matrix as a noise adaptation layer with fixed parameters, with a total of $c^2$ parameters, where $c$ represents the number of categories. However, the number of parameters in a deep neural network is significantly greater. Taking Resnet-18 as an example, it has a total of 11.7M parameters. Therefore, in this paper and in most cases, we have $T << P$ and $T << E$. Consequently, we can simplify the two computational complexities to $O(4eT + (c+e)P)$ and $O(2eT + P)$. Since the training process involves backpropagation and gradient computation, it takes more time than the prediction process, leading to $T > P$. Additionally, in this paper, the number of pruning iterations satisfies $e \gg c$. As a result, the computational complexity of the proposed method follows $O(4eT + (c+e)P) < O(6eT)$, and the Forward follows $O(2eT + P) > O(2eT)$. Hence, under the assumption of setting the same number of epochs in each stage, the time overhead of the proposed method should be less than three times that of the Forward. Additionally, for the purpose of evaluating the efficiency of our approach, we conducted a comparison of the code's runtime based on the CIFAR-10 dataset.
\begin{table}[htb]
    % \scriptsize
    \caption{The classification accuracy (expressed in percentage) with different cropping size (number of features).}
    \label{tab:time}
    \centering
    \begin{tabular}{cc}
      \toprule
      Method & Time Consumption (min) \\ 
      \midrule
      PLM & 35.56\\
      Forward & 19.21\\
      \bottomrule
    \end{tabular}
  \end{table}

Analysis and experiments indicate that our approach significantly enhances the performance of LNL, with only a linear increase in time consumption.

\section{Hyperparameter sensitivity analysis}
The instance cropping method is related to the multi-labeling of the proposed approach. In the paper, we selected the four corners and the central part of the image data for cropping and determined the cropping size through empirical analysis on the validation set. Table \ref{tab:cropping} displays the experimental results of different cropping sizes on CIFAR-10 data with sym-50\% noise, and we additionally attempted two other cropping strategies. The cropping strategies used in table \ref{tab:cropping} are as follows: the uniform strategy involves five uniform crops at the four corners and center of the image as used in the paper. The random strategy entails five crops at random positions. The emphasized strategy constructs two sub-instances based on feature emphasis, with one sub-instance masking the top emphasized number of features and the other sub-instance masking the remaining features. 
\begin{table}[htb]
  % \scriptsize
  \caption{The classification accuracy (expressed in percentage) with different cropping size (number of features).}
  \label{tab:cropping}
  \centering
  \begin{tabular}{cccc}
    \toprule
    Size&Uniform & Random & Emphasized \\ 
    \midrule
    9 & $83.58\pm0.45$ & $83.42\pm0.86$  & $84.14\pm0.59$\\
    36 & $83.80\pm0.31$ & $83.40\pm0.55$ & $84.24\pm0.29$\\
    81 & $82.69\pm2.32$ & $83.81\pm0.54$ & $84.48\pm0.47$\\
    144 & $83.17\pm0.91$ &  $83.81\pm0.39$& $84.19\pm0.42$\\
    256 & $83.49\pm0.95$ & $83.40\pm0.34$ & $84.28\pm0.86$\\
    361 & $83.62\pm0.31$ & $83.65\pm0.74$ & $84.32\pm0.46$\\
    484 & $84.99\pm0.40$ & $84.36\pm0.32$ & $84.24\pm0.61$\\
    625 & $85.08\pm0.16$ & $83.97\pm0.72$ & $84.26\pm0.57$\\
    784 & $84.24\pm0.24$ & $83.91\pm0.70$ & $84.47\pm0.33$\\
    \bottomrule
  \end{tabular}
\end{table}

The emphasized strategy demonstrates superior performance and displays enhanced stability, suggesting the potential for further refinement of cropping strategies in the context of LNL classification, as discussed in Section 5 of the paper. Furthermore, within the established cropping strategy, the method shows robustness to the cropping size.
\begin{table*}[htb]
  \caption{The average classification accuracy and standard deviation (expressed in percentage) across five trials on the CIFAR-10 dataset.}
  \label{tab:accuracy-10}
  \centering
  \begin{tabular}{ccccc}
    \toprule
    % \multicolumn{5}{c}{MNIST}\\
     & Sym-20\% & Sym-50\% & Pair-20\% & Pair-45\% \\    
    \midrule
    Forward & $85.62\pm0.58$ & $73.78\pm0.99$ & $89.20\pm1.56$ & $66.20\pm10.05$ \\
    PLM-F & \boldmath{$89.45\pm0.59$} & \boldmath{$81.94\pm0.62$} & \boldmath{$91.29\pm0.18$} & \boldmath{$74.90\pm1.37$} \\
    \midrule
    Dual-T & $89.79\pm0.40$ & $77.97\pm1.91$ & $89.63\pm1.38$ & $60.57\pm10.72$ \\
    PLM-D & \boldmath{$90.95\pm0.28$} & \boldmath{$85.38\pm0.49$} & \boldmath{$93.15\pm0.26$} & \boldmath{$91.10\pm2.17$} \\
    \midrule
    T-Revision & $88.68\pm0.54$ & $82.59\pm1.82$ & $91.10\pm0.21$ & $72.65\pm16.11$ \\
    PLM-R & \boldmath{$91.33\pm0.47$} & \boldmath{$85.22\pm0.54$} & \boldmath{$92.69\pm0.23$} & \boldmath{$91.33\pm0.60$} \\
    \midrule
    VolMinNet & $90.19\pm0.17$ & $84.09\pm0.68$ & $91.55\pm0.13$ & $86.12\pm1.26$ \\
    PLM-V & \boldmath{$91.75\pm0.19$} & \boldmath{$84.10\pm0.55$} & \boldmath{$93.40\pm0.23$} & \boldmath{$86.91\pm1.02$} \\
    \bottomrule
  \end{tabular}
\end{table*}
\begin{table*}[htb]
  \caption{The average classification accuracy and standard deviation (expressed in percentage) across five trials on the CIFAR-100 dataset.}
  \label{tab:accuracy-100}
  \centering
  \begin{tabular}{ccccc}
    \toprule
     & Sym-20\% & Sym-50\% & Pair-20\% & Pair-45\% \\
    \midrule
    Forward & $58.70\pm0.73$ & $39.82\pm2.15$ & $60.12\pm0.33$ & $37.99\pm0.37$ \\
    PLM-F & \boldmath{$68.19\pm0.92$} & \boldmath{$58.59\pm0.92$} & \boldmath{$70.94\pm1.16$} & \boldmath{$55.47\pm1.27$} \\
    \midrule
    Dual-T & $65.62\pm0.39$ & $50.07\pm1.56$ & $71.08\pm0.27$ & $52.25\pm3.28$ \\
    PLM-D & \boldmath{$69.44\pm0.27$} & \boldmath{$60.84\pm0.38$} & \boldmath{$71.90\pm0.56$} & \boldmath{$68.38\pm1.11$} \\
    \midrule
    T-Revision & $61.14\pm0.69$ & $40.01\pm0.90$ & $60.56\pm0.66$ & $49.44\pm1.64$ \\
    PLM-R & \boldmath{$67.52\pm1.19$} & \boldmath{$50.81\pm3.31$} & \boldmath{$70.58\pm1.13$} & \boldmath{$56.85\pm1.73$} \\
    \midrule
    VolMinNet & $67.70\pm0.99$ & $57.99\pm0.40$ & $71.65\pm0.62$ & $61.21\pm2.98$ \\
    PLM-V & \boldmath{$70.95\pm0.49$} & \boldmath{$62.37\pm0.29$} & \boldmath{$74.55\pm0.12$} & \boldmath{$64.05\pm0.53$} \\
    \bottomrule
  \end{tabular}
\end{table*}

\section{The experimental results with different noise transition matrix estimation} \label{sec:matrix}
In the main paper (Section 5), we presented the experimental results of on the CIFAR-10 and CIFAR-100 datasets. As an extension to this research, this section aims to compare the outcomes achieved by our proposed method when integrated with various noise transition matrix estimation techniques. In the main paper, we followed the approach outlined in Forward \cite{patrini2017making} to select specific percentiles as anchor points. However, this selection method may not be universally applicable \cite{yao2020dual}. Therefore, in this experiment, we compare the results by employing a sample with the highest probability as the anchor point for each class. 

We have conducted a comparison of performance using various matrix estimation methods. More specifically, for PLM-F, PLM-D, and PLM-V, we adopted the matrix estimation techniques outlined in Forward \cite{patrini2017making}, Dual-T \cite{yao2020dual}, and VolMinNet \cite{li2021provably}, respectively. Subsequently, we minimize the empirical risk as defined in \eq{eq:risk}. For PLM-R, we combined PLM with T-Revision \cite{xia2019anchor} and introduced the slack variable $\Delta T$, then $f^e(\boldsymbol{x})$ in Eq. \eqref{eq:eqfe} can be modified to 
\begin{equation}
    f^{er}(\boldsymbol{x})=\arg\max_{i \in \{1,\cdots,c\}}((T(\boldsymbol{x})+\Delta T)g)_i(\boldsymbol{x}).
\end{equation}
Following T-Revision, we also incorporated a importance reweighting strategy. The minimized empirical risk of PLM-R is defined as follows:
\begin{equation}
  \hat{R}(f^{er},f^p)=\frac{1}{2n}\sum_{i=1}^{n}[w\ell_1(f^{er}(\boldsymbol{x}_i),\tilde{y}_i)+\ell_2(f^p(\boldsymbol{x}_i),\boldsymbol{y}^\prime_i)],
\end{equation}
where weight $w = \frac{g_{y_i}(\boldsymbol{x}_i)}{((T(\boldsymbol{x})+\Delta T)g)_{y_i}(\boldsymbol{x}_i)}$.

In table \ref{tab:accuracy-10} and table \ref{tab:accuracy-100}, we bold the better classification accuracy. The results demonstrate that our proposed method can serve as a component to enhance the robustness of the loss correction methods.

\begin{figure}[htb]
  \centering
  \begin{minipage}[t]{\linewidth}
    \centering
    \begin{minipage}[t]{0.135\linewidth}
      \centering
      \includegraphics[width=\linewidth]{./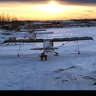}
    \end{minipage}
    \hspace{0.01\linewidth}
    \begin{minipage}[t]{0.135\linewidth}
      \centering
      \includegraphics[width=\linewidth]{./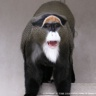}
    \end{minipage}
    \hspace{0.01\linewidth}
    \begin{minipage}[t]{0.135\linewidth}
      \centering
      \includegraphics[width=\linewidth]{./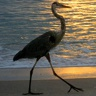}
    \end{minipage}
    \hspace{0.01\linewidth}
    \begin{minipage}[t]{0.135\linewidth}
      \centering
      \includegraphics[width=\linewidth]{./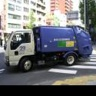}
    \end{minipage}
    \hspace{0.01\linewidth}
    \begin{minipage}[t]{0.135\linewidth}
      \centering
      \includegraphics[width=\linewidth]{./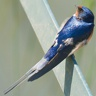}
    \end{minipage}
    \hspace{0.01\linewidth}
    \begin{minipage}[t]{0.135\linewidth}
      \centering
      \includegraphics[width=\linewidth]{./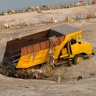}
    \end{minipage}
  \subcaption{}\label{fig:cam1}
  \end{minipage}
  \begin{minipage}[t]{\linewidth}
    \centering
    \begin{minipage}[t]{0.135\linewidth}
      \centering
      \includegraphics[width=\linewidth]{./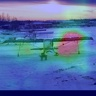}
    \end{minipage}
    \hspace{0.01\linewidth}
    \begin{minipage}[t]{0.135\linewidth}
      \centering
      \includegraphics[width=\linewidth]{./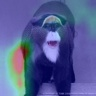}
    \end{minipage}
    \hspace{0.01\linewidth}
    \begin{minipage}[t]{0.135\linewidth}
      \centering
      \includegraphics[width=\linewidth]{./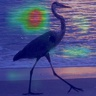}
    \end{minipage}
    \hspace{0.01\linewidth}
    \begin{minipage}[t]{0.135\linewidth}
      \centering
      \includegraphics[width=\linewidth]{./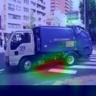}
    \end{minipage}
    \hspace{0.01\linewidth}
    \begin{minipage}[t]{0.135\linewidth}
      \centering
      \includegraphics[width=\linewidth]{./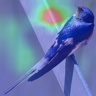}
    \end{minipage}
    \hspace{0.01\linewidth}
    \begin{minipage}[t]{0.135\linewidth}
      \centering
      \includegraphics[width=\linewidth]{./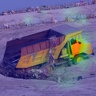}
    \end{minipage}
    \subcaption{}\label{fig:cam2}
  \end{minipage}
  \begin{minipage}[t]{\linewidth}
    \centering
    \begin{minipage}[t]{0.135\linewidth}
      \centering
      \includegraphics[width=\linewidth]{./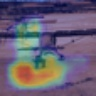}
    \end{minipage}
    \hspace{0.01\linewidth}
    \begin{minipage}[t]{0.135\linewidth}
      \centering
      \includegraphics[width=\linewidth]{./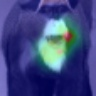}
    \end{minipage}
    \hspace{0.01\linewidth}
    \begin{minipage}[t]{0.135\linewidth}
      \centering
      \includegraphics[width=\linewidth]{./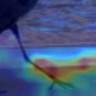}
    \end{minipage}
    \hspace{0.01\linewidth}
    \begin{minipage}[t]{0.135\linewidth}
      \centering
      \includegraphics[width=\linewidth]{./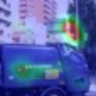}
    \end{minipage}
    \hspace{0.01\linewidth}
    \begin{minipage}[t]{0.135\linewidth}
      \centering
      \includegraphics[width=\linewidth]{./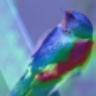}
    \end{minipage}
    \hspace{0.01\linewidth}
    \begin{minipage}[t]{0.135\linewidth}
      \centering
      \includegraphics[width=\linewidth]{./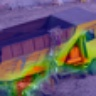}
    \end{minipage}
    \subcaption{}\label{fig:cam3}
  \end{minipage}
  \begin{minipage}[t]{\linewidth}
    \centering
    \begin{minipage}[t]{0.135\linewidth}
      \centering
      \includegraphics[width=\linewidth]{./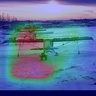}
    \end{minipage}
    \hspace{0.01\linewidth}
    \begin{minipage}[t]{0.135\linewidth}
      \centering
      \includegraphics[width=\linewidth]{./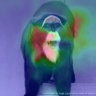}
    \end{minipage}
    \hspace{0.01\linewidth}
    \begin{minipage}[t]{0.135\linewidth}
      \centering
      \includegraphics[width=\linewidth]{./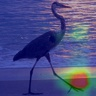}
    \end{minipage}
    \hspace{0.01\linewidth}
    \begin{minipage}[t]{0.135\linewidth}
      \centering
      \includegraphics[width=\linewidth]{./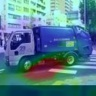}
    \end{minipage}
    \hspace{0.01\linewidth}
    \begin{minipage}[t]{0.135\linewidth}
      \centering
      \includegraphics[width=\linewidth]{./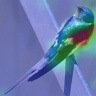}
    \end{minipage}
    \hspace{0.01\linewidth}
    \begin{minipage}[t]{0.135\linewidth}
      \centering
      \includegraphics[width=\linewidth]{./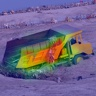}
    \end{minipage}
    \subcaption{}\label{fig:cam4}
  \end{minipage}
  
  \caption{Illustration of class activation maps (CAM) for overemphasized region correction: the highlighted area (with more intense red color) indicates the emphasized area of a model trained from noisy labels. (a) Original images with noisy labels: car, bird, dog, monkey, ship, deer. (b) CAMs for estimating noisy class posterior by the classifier.  (c) CAMs when excluding the overemphasized regions after cropping. (d) CAMs for estimating noisy class posterior by the model after PLM training.} \label{fig:cam}
\end{figure} 

\section{Visualization of focused features}
In Figure \ref{fig:cam}, we employ a visualization approach to provide a visual interpretation of the effectiveness of the PLM method. The STL-10 \cite{coates2011analysis} dataset is used for visualization purposes. In Figure \ref{fig:cam2}, it is shown that when the labels contain noise, the network emphasizes the background region associated with those labels. Consequently, the model tends to overfit to the noise, hindering the network's ability to learn features that truly capture the distinctive characteristics of the instances. As a result, the estimation of the posterior for the noisy labels becomes excessively confident. As depicted in Figure \ref{fig:cam3}, removing the overemphasized features through cropping effectively redirects the model's attention to other more informative features. By generating labels associated with these features and providing additional supervisory information during network training, the network can focus on more diverse features. As shown in Figure \ref{fig:cam4}, compared to Figure \ref{fig:cam2}, the network pays more attention to object-relevant features.

% \clearpage
% \setcounter{page}{1}
% \maketitlesupplementary

% \section{Rationale}
% \label{sec:rationale}
% % 
% Having the supplementary compiled together with the main paper means that:
% % 
% \begin{itemize}
% \item The supplementary can back-reference sections of the main paper, for example, we can refer to \cref{sec:intro};
% \item The main paper can forward reference sub-sections within the supplementary explicitly (e.g. referring to a particular experiment); 
% \item When submitted to arXiv, the supplementary will already included at the end of the paper.
% \end{itemize}
% % 
% To split the supplementary pages from the main paper, you can use \href{https://support.apple.com/en-ca/guide/preview/prvw11793/mac#:~:text=Delete%20a%20page%20from%20a,or%20choose%20Edit%20%3E%20Delete).}{Preview (on macOS)}, \href{https://www.adobe.com/acrobat/how-to/delete-pages-from-pdf.html#:~:text=Choose%20%E2%80%9CTools%E2%80%9D%20%3E%20%E2%80%9COrganize,or%20pages%20from%20the%20file.}{Adobe Acrobat} (on all OSs), as well as \href{https://superuser.com/questions/517986/is-it-possible-to-delete-some-pages-of-a-pdf-document}{command line tools}.
